# Supplementary material for: Universal Approximation Theorems for Differentiable Geometric Deep Learning
Source: arXiv:2101.05390 source file (2022-07-25)
Supplement: Supplementary file 1 [file 4_Future_Research.tex]

\section*{Future research}
Beyond the tools for building universal approximators with quantifiable performance suited to specific learning tasks, our findings raise several broader questions. We briefly outline some of these questions, which are to be the subject of future investigation.  

\hfill\\
\noindent \textbf{Optimal the width to depth ratios.} 
As described in Remark~\ref{r_narrow_vs_deep}, there is a non-trivial relationship between width and depth which has been optimized for deep ReLU networks between Euclidean geometry in \cite{pmlrv75yarotsky18a}.  Our findings suggest the question \textit{what is the optimal depth-to-width ratio} both as a function of the unknown function's regularity and the local geometries of the input and output spaces. 

\hfill\\
\noindent \textbf{Quantitative Approximation for Other Topologies}
Another direction for future work is to extend the quantitative approximation results of classical feedforward networks, for functions lying in Sobolev spaces, as obtained in \cite{Yarotski,QuantitativeDeepReLUSobolev,YAROTSKYSobolev,SIEGEL2020313}, or lying in Besov spaces, as obtained in \cite{Besov,gribonval2019approximation}, to approximation results for GDNs between a broader class metric input output spaces.  A likely point of continuation would be to exploit the well-developed literature of Sobolev spaces between metric-measures spaces, as pioneered in \cite{KorevaarSchoen1993,PiotsPekkaClassic1995Pointcareinequalityweak,HajlaszsobolMMs1996}, or the theory flourishing literature of Besov spaces with such inputs and outputs, see \cite{BesovMMs2008}.  

\hfill\\
\noindent \textbf{Non-null homotopic functions.} Theorems~\ref{thrm_homotopic_necessary_condition} and~\ref{thrm_negative_motiation} and their consequence open the way to the investigation of non-null homotopic deep neural models. Nevertheless, the construction of such networks and a method for efficiently training them is an interesting future research challenge since the recent computational topology results of \cite{MR3268623,matousek2013computing} shows that a even a computation of the possible homotopy types of a Riemannian output space is a computational challenge, of at-least $P$ complexity.
